# Supplementary material for: Estimating Bethe roots with VQE
Source: arXiv:2404.18244 source file (2024-08-11)
Supplement: Supplementary file 1 [file BetheVQEOpen_arxiv1.pdf]

# BetheVQEOpen_arxiv1

April 28, 2024

## 1 Estimating Bethe roots for the open spin-1/2 XXZ chain using VQE

[1]:
```
pip install qiskit-nature
```

```
Requirement already satisfied: qiskit-nature in /opt/conda/lib/python3.10/site-
packages (0.7.2)
Requirement already satisfied: qiskit>=0.44 in /opt/conda/lib/python3.10/site-
packages (from qiskit-nature) (1.0.2)
Requirement already satisfied: qiskit-algorithms>=0.2.1 in
/opt/conda/lib/python3.10/site-packages (from qiskit-nature) (0.3.0)
Requirement already satisfied: scipy>=1.4 in /opt/conda/lib/python3.10/site-
packages (from qiskit-nature) (1.12.0)
Requirement already satisfied: numpy>=1.17 in /opt/conda/lib/python3.10/site-
packages (from qiskit-nature) (1.23.5)
Requirement already satisfied: psutil>=5 in /opt/conda/lib/python3.10/site-
packages (from qiskit-nature) (5.9.4)
Requirement already satisfied: setuptools>=40.1.0 in
/opt/conda/lib/python3.10/site-packages (from qiskit-nature) (65.5.1)
Requirement already satisfied: typing-extensions in
/opt/conda/lib/python3.10/site-packages (from qiskit-nature) (4.9.0)
Requirement already satisfied: h5py in /opt/conda/lib/python3.10/site-packages
(from qiskit-nature) (3.7.0)
Requirement already satisfied: rustworkx>=0.12 in
/opt/conda/lib/python3.10/site-packages (from qiskit-nature) (0.14.0)
Requirement already satisfied: sympy>=1.3 in /opt/conda/lib/python3.10/site-
packages (from qiskit>=0.44->qiskit-nature) (1.11.1)
Requirement already satisfied: dill>=0.3 in /opt/conda/lib/python3.10/site-
packages (from qiskit>=0.44->qiskit-nature) (0.3.6)
Requirement already satisfied: python-dateutil>=2.8.0 in
/opt/conda/lib/python3.10/site-packages (from qiskit>=0.44->qiskit-nature)
(2.8.2)
Requirement already satisfied: stevedore>=3.0.0 in
/opt/conda/lib/python3.10/site-packages (from qiskit>=0.44->qiskit-nature)
(5.1.0)
Requirement already satisfied: symengine>=0.11 in
/opt/conda/lib/python3.10/site-packages (from qiskit>=0.44->qiskit-nature)
(0.11.0)
```

```
Requirement already satisfied: six>=1.5 in /opt/conda/lib/python3.10/site-
packages (from python-dateutil>=2.8.0->qiskit>=0.44->qiskit-nature) (1.16.0)
Requirement already satisfied: pbr!=2.1.0,>=2.0.0 in
/opt/conda/lib/python3.10/site-packages (from
stevedore>=3.0.0->qiskit>=0.44->qiskit-nature) (6.0.0)
Requirement already satisfied: mpmath>=0.19 in /opt/conda/lib/python3.10/site-
packages (from sympy>=1.3->qiskit>=0.44->qiskit-nature) (1.2.1)
Note: you may need to restart the kernel to use updated packages.
```

[2]:
```
pip install qiskit_algorithms
```

```
Requirement already satisfied: qiskit_algorithms in
/opt/conda/lib/python3.10/site-packages (0.3.0)
Requirement already satisfied: qiskit>=0.44 in /opt/conda/lib/python3.10/site-
packages (from qiskit_algorithms) (1.0.2)
Requirement already satisfied: scipy>=1.4 in /opt/conda/lib/python3.10/site-
packages (from qiskit_algorithms) (1.12.0)
Requirement already satisfied: numpy>=1.17 in /opt/conda/lib/python3.10/site-
packages (from qiskit_algorithms) (1.23.5)
Requirement already satisfied: rustworkx>=0.14.0 in
/opt/conda/lib/python3.10/site-packages (from qiskit>=0.44->qiskit_algorithms)
(0.14.0)
Requirement already satisfied: sympy>=1.3 in /opt/conda/lib/python3.10/site-
packages (from qiskit>=0.44->qiskit_algorithms) (1.11.1)
Requirement already satisfied: dill>=0.3 in /opt/conda/lib/python3.10/site-
packages (from qiskit>=0.44->qiskit_algorithms) (0.3.6)
Requirement already satisfied: python-dateutil>=2.8.0 in
/opt/conda/lib/python3.10/site-packages (from qiskit>=0.44->qiskit_algorithms)
(2.8.2)
Requirement already satisfied: stevedore>=3.0.0 in
/opt/conda/lib/python3.10/site-packages (from qiskit>=0.44->qiskit_algorithms)
(5.1.0)
Requirement already satisfied: typing-extensions in
/opt/conda/lib/python3.10/site-packages (from qiskit>=0.44->qiskit_algorithms)
(4.9.0)
Requirement already satisfied: symengine>=0.11 in
/opt/conda/lib/python3.10/site-packages (from qiskit>=0.44->qiskit_algorithms)
(0.11.0)
Requirement already satisfied: six>=1.5 in /opt/conda/lib/python3.10/site-
packages (from python-dateutil>=2.8.0->qiskit>=0.44->qiskit_algorithms) (1.16.0)
Requirement already satisfied: pbr!=2.1.0,>=2.0.0 in
/opt/conda/lib/python3.10/site-packages (from
stevedore>=3.0.0->qiskit>=0.44->qiskit_algorithms) (6.0.0)
Requirement already satisfied: mpmath>=0.19 in /opt/conda/lib/python3.10/site-
packages (from sympy>=1.3->qiskit>=0.44->qiskit_algorithms) (1.2.1)
Note: you may need to restart the kernel to use updated packages.
```

[3]:
```python
import qiskit

qiskit.version.get_version_info()
```

[3]: '1.0.2'

## 1.1 Function $f(w,k)$ for *open*

Make the function $f(w,k)$ for a given set of Bethe roots $\vec{k}$

$$f(w,\vec{k}) = \sum_{\sigma\in S_M}\sum_{\epsilon_1,\ldots,\epsilon_M=\pm 1} \varepsilon(\sigma)\,\epsilon_1\ldots\epsilon_M\,A(\epsilon_1 k_{\sigma(1)},\ldots,\epsilon_M k_{\sigma(M)})\,e^{i\sum_{j=1}^{M}\epsilon_j k_{\sigma(j)} x_j}$$

$$A(k_1,\ldots,k_M) = \prod_{j=1}^{M}\beta(-k_j)\prod_{1\le j<l\le M} B(-k_j,k_l)\,e^{-ik_l}$$

$$B(k,k') = s(k,k')\,s(k',-k)$$

$$s(k,k') = 1-2\Delta e^{ik'} + e^{i(k+k')}$$

$$\alpha(k) = 1+(h-\Delta)\,e^{-ik}\,, \qquad \beta(k) = \left[1+(h'-\Delta)\,e^{-ik}\right]e^{i(L+1)k}$$

[4]:
```python
import numpy as np
import math
import itertools
np.set_printoptions(suppress=True)
np.set_printoptions(threshold=np.inf)
```

[5]:
```python
# mylist is a collection of permutations t of the numbers 0 to M-1
def mylist(M):
    return list(itertools.permutations(range(M)))

# mysign gives all possible choices of [e0,e1,...,eM-1], where e=\pm 1
def mysign(M):
    return list(itertools.product([-1,1],repeat=M))

# gives all permutations w
def allperm(L,M):
    u=[0]*(L-M)+[1]*M
    return list(set(itertools.permutations(u)))

# inversion number of t=(0,1,2,...,M-1)
def inv(t):
    x=0
    for j in range(M):
```

```
        for i in range(j):
            if t[i]>t[j]:
                x=x+1
    return x

# sign of permutation t
def e(t):
    return (-1)**inv(t)

def s(k,kp):
    return 1-2*Delta*np.exp(1.j*kp)+np.exp(1.j*(k+kp))

def B(k,kp):
    return s(k,kp)*s(kp,-k)

def beta(k):
    return (1+(hp-Delta)*np.exp(-1j*k))*np.exp(1j*(L+1)*k)

# k=[k0,...,kM-1]
def A(k,sign):
    x=1
    for l in range(len(k)):
        x=x*beta(-sign[l]*k[l])
    for l in range(len(k)):
        for j in range(l):
            x=x*B(-sign[j]*k[j],sign[l]*k[l])*np.exp(-1j*sign[l]*k[l])
    return x

# permutes the bethe roots k into an order determined by t: [k0,k1,k2] ->
  ↪[k1,k2,k0]
def kperm(k,t):
    y=[]
    for i in t:
        y.append(k[i])
    return y

# positions of the ones in w
def positions(w):
    x=[]
    for i in range(len(w)):
        if w[i]==1:
            x.append(i+1) # positions run from 1 to L, not 0 to L-1
    return x

def f(w,k):
    x=positions(w)
    z=0
```

```
    for sign in mysign(len(k)): # all negations of bethe roots
        numnegatives=0
        for i in sign:
            if i==-1:
                numnegatives=numnegatives+1
        for t in mylist(len(k)): # all permutations of bethe roots
            y=kperm(k,t)
            v=0
            for i in range(len(k)):
                v=v+sign[i]*y[i]*x[i]
            v=np.exp(1.j*v)
            z=z+e(t)*((-1)**numnegatives)*A(y,sign)*v
    return z
```

## 1.2 Hamiltonian

$$\mathcal{H} = \frac{1}{4}\sum_{n=1}^{L-1}\left(\sigma_n^x\sigma_{n+1}^x + \sigma_n^y\sigma_{n+1}^y + \Delta\,\sigma_n^z\sigma_{n+1}^z\right) + \frac{1}{4}\left(h\,\sigma_1^z + h'\,\sigma_L^z\right)$$

[22]:
```
L=3
M=2
Delta=0.5
h=3
hp=0.3
```

[7]:
```
from qiskit_nature.second_q.hamiltonians.lattices import (
    BoundaryCondition,
    Lattice,
    LatticeDrawStyle,
    LineLattice,
)
from qiskit_nature.second_q.hamiltonians import HeisenbergModel
from qiskit_nature.second_q.mappers import LogarithmicMapper
from qiskit.quantum_info import Pauli, SparsePauliOp
```

[8]:
```
#bulk terms in Hamiltonian

num_nodes=L
ham_bulk_sop = HeisenbergModel(LineLattice(num_nodes,␣
 ↪boundary_condition=BoundaryCondition.OPEN), (1.0, 1.0, Delta), (0.0, 0.0, 0.
 ↪0))

logmapper = LogarithmicMapper()

ham_bulk_op=logmapper.map(ham_bulk_sop.second_q_op())

#boundary terms in Hamiltonian
```

```
btL=Pauli(([0]*(L-1)+[1],[0]*L))
opL=SparsePauliOp(btL.to_label(), coeffs=[h/4.0])

btR=Pauli(([1]+[0]*(L-1),[0]*L))
opR=SparsePauliOp(btR.to_label(), coeffs=[hp/4.0])

ham_bound_op = opL + opR
ham = ham_bulk_op + ham_bound_op
hamsquared =  ham @ ham
```

[78]:
```
#ham.to_matrix()
```

## 1.3 Variational ansatz

[9]:
```
from qiskit import *
from qiskit import QuantumRegister
from qiskit import QuantumCircuit
from qiskit.circuit.library import RYGate
from qiskit.circuit.library import UGate
np.set_printoptions(suppress=True)
np.set_printoptions(threshold=np.inf)
```

[10]:
```
from qiskit.circuit import ParameterVector
```

Among the “kparts” cells below, ONLY ONE CELL SHOULD BE RUN!

If you are searching for all real roots, only the first cell is run, etc.

[11]:
```
# M real roots
kparts = ParameterVector("kparts", M)
k=kparts
```

[15]:
```
# one complex root, M=1
kparts = ParameterVector("kparts",2)
k=[kparts[0]+1j*kparts[1]]
```

[28]:
```
# one complex root, one real root, M=2
kparts = ParameterVector("kparts",3)
k=[kparts[0]+1j*kparts[1],kparts[2]]
```

[23]:
```
# one complex root, one purely imaginary root, M=2
kparts = ParameterVector("kparts",3)
k=[kparts[0]+1j*kparts[1],1j*kparts[2]]
```

[14]:
```
# one complex root, 3 real roots, M=4
kparts = ParameterVector("kparts",5)
k=[kparts[0]+1j*kparts[1],kparts[2],kparts[3],kparts[4]]
```

## 1.4 Bethe Circuit

Prepares the Bethe state

$$|B_M^L(\vec{k})\rangle = \sum_{w\in P(L,M)} f(w,\vec{k})\,|w\rangle$$

[29]:
```python
q=QuantumRegister(L)
bethe = QuantumCircuit(q)

# Create set of permutations
def P(L,M):
    if M==0:
        return [[0] * L]
    elif L-M==0:
        return [[1] * L]
    else:
        x=[]
        for p0 in P(L-1,M):
            x.append(p0+[0])
        for p1 in P(L-1,M-1):
            x.append(p1+[1])
        return x

# store the coefficients f(w,k)
farray=[]
for w in P(L,M):
    farray=farray+[[w,f(w,k)]]

def F(b):
    sol=[] # solutions of w=ab
    for w in P(L,M):
        if w[L-len(b):L]==b:
            sol.append(w)
    if len(sol)==1:
        position=P(L,M).index(sol[0])
        return farray[position][1]
    else:
        x=0
        for p in sol:
            position=P(L,M).index(p)
            x=x+abs(farray[position][1])**2
        return x**0.5

def G(i,b):
    x=[i] + b
    return F(x)/F(b)
```

```
# a way of obtaining the angle arg(x) when x is a ParameterExpression
def myangle(x):
    eps=1e-16j
    y = -1j*np.log(x/np.abs(x)+eps)
    return (y+np.conjugate(y))/2

def theta(b):
    return 2*np.arccos(abs(G(1,b)))
def lam(b):
    return myangle(G(0,b)) -np.pi
def phi(b):
    return myangle(G(1,b))-lam(b)

def u(b):
    t=theta(b)
    la=lam(b)
    p=phi(b)
    return UGate(t,p,la)

def applyX(m,l):
    bethe.cx(L-m,L-m+l)

def applyI(m,l):
    sol=[] # these will be the strings b in P(L-m,M-l)
    for b in P(L-m,M-l):
        if F(b)!=0: # Check that F(b)!=0
            sol.append(b)
    if len(sol)==1:
        applyX(m,l)
        b=sol[0] # when b is unique, no extra controls are needed
        if l==1:
            cU = u(b).control(1)
            bethe.append(cU,[L-m+l,L-m])
        else:
            ccU = u(b).control(2)
            bethe.append(ccU,[L-m+l-1,L-m+l,L-m])
        applyX(m,l)
    elif len(sol)>1:
        applyX(m,l)
        for b in sol:
            extra=[] # these are going to be the locations of the extra controls
            for i in range(len(b)):
                if b[i]==1:
                    # if b=[0,1] then extra=[0], location of control
                    extra.append(len(b)-i-1)
            if l==1:
```

```
                cU = u(b).control(1+len(extra))
                bethe.append(cU,extra + [L-m+l,L-m])
            else:
                ccU = u(b).control(2+len(extra))
                bethe.append(ccU,extra + [L-m+l-1,L-m+l,L-m])
        applyX(m,l)

# Create initial state
for i in range(M):
    bethe.x(i)
bethe.barrier()

# Apply I-gates
for m in reversed(range(2,L+1)):
    for l in range(max(M+m-L,1),min(M,m-1)+1):
        print(m,l)
        applyI(m,l)
    bethe.barrier()

#bethe.draw(output='mpl', initial_state=True)
```

```
3 2
2 1
```

[13]:

```
#print(ham)
#ham.to_matrix()
```

Prints the minimum eigenvalue of our Hamiltonian

[25]:

```
from qiskit_algorithms import NumPyMinimumEigensolver

numpy_solver = NumPyMinimumEigensolver()
result = numpy_solver.compute_minimum_eigenvalue(operator=ham)
ref_value = result.eigenvalue.real
print(ref_value)
```

```
-1.4950599509876246
```

### 1.5 Statevector VQE: Ground state

[30]:

```
from qiskit.primitives import Estimator
from qiskit_algorithms.utils import algorithm_globals
from qiskit_aer.primitives import Estimator as AerEstimator

estimator = Estimator()

# define optimizer
from qiskit_algorithms.optimizers import SLSQP, COBYLA
iterations = 1000
```

```
optimizer = SLSQP(maxiter=iterations)
cobyla= COBYLA(maxiter=1000)

from qiskit_algorithms import VQE
# define callback
# note: Re-run this cell to restart lists before training
counts = []
values = []

def store_intermediate_result(eval_count, parameters, mean, std):
    counts.append(eval_count)
    values.append(mean)
```

[31]:

```
x0=np.random.uniform(0,np.pi,bethe.num_parameters)

print(x0)

vqe = VQE(estimator, bethe, cobyla, callback=store_intermediate_result,␣
 ↪initial_point=x0)
result = vqe.compute_minimum_eigenvalue(operator=ham)

print(result)
```

```
[3.07876544 2.0675507  2.36419917]
{   'aux_operators_evaluated': None,
    'cost_function_evals': 179,
    'eigenvalue': -1.495059834265502,
    'optimal_circuit': <qiskit.circuit.quantumcircuit.QuantumCircuit object at
0x7f250186c340>,
    'optimal_parameters': {   ParameterVectorElement(kparts[0]):
3.140155880028671,
                              ParameterVectorElement(kparts[1]):
0.9106702312271622,
                              ParameterVectorElement(kparts[2]):
1.6988460766148958},
    'optimal_point': array([3.14015588, 0.91067023, 1.69884608]),
    'optimal_value': -1.495059834265502,
    'optimizer_evals': None,
    'optimizer_result': <qiskit_algorithms.optimizers.optimizer.OptimizerResult
object at 0x7f2501651330>,
    'optimizer_time': 5.8836283683776855}
```

### 1.6 Statevector VQE: Variance

[18]:

```
# define Estimator for exact statevector simulation
from qiskit.primitives import StatevectorEstimator as Estimator
```

```
estimator = Estimator()

# define optimizer
from qiskit_algorithms.optimizers import SLSQP, COBYLA
iterations = 1000
optimizer = SLSQP(maxiter=iterations)
cobyla= COBYLA(maxiter=1000)

from qiskit_algorithms import VQE
```

[19]:
```
def evaluate_var(params):
    estimator_job1 = estimator.run([(bethe, hamsquared, params)])
    estimator_job2 = estimator.run([(bethe, ham, params)])
    estimator_result1  = estimator_job1.result()
    estimator_result2  = estimator_job2.result()
    er1=estimator_result1[0].data.evs
    er2=estimator_result2[0].data.evs
    var =  er1  -  er2**2
    return var

x0=np.random.uniform(0,np.pi,bethe.num_parameters)

print(x0)
opt_result = cobyla.minimize(evaluate_var, x0)
print(opt_result)
```

```
[2.93378481 2.22561589]
{   'fun': 1.6766638077925222e-09,
    'jac': None,
    'nfev': 43,
    'nit': None,
    'njev': None,
    'x': array([3.14168748, 0.91138529])}
```

### 1.7 Shots VQE: Ground state

[32]:
```
from qiskit_aer.primitives import Estimator as AerEstimator

aer_estimator = AerEstimator(run_options={"shots": 10000})

def evaluate_energy(x0):
    estimator_job1 = aer_estimator.run(bethe.assign_parameters({kparts: x0}),␣
 ↪ham)
    estimator_result1  = estimator_job1.result()
    return estimator_result1.values
```

[33]:
```
from qiskit_algorithms.optimizers import COBYLA

cobyla = COBYLA()

x0=np.random.uniform(0,np.pi,bethe.num_parameters)

print(x0)
opt_result = cobyla.minimize(evaluate_energy, x0)
print(opt_result)
```

```
[3.07607891 1.04083885 1.60008922]
{   'fun': -1.4841099999999998,
    'jac': None,
    'nfev': 41,
    'nit': None,
    'njev': None,
    'x': array([3.34181259, 0.95904005, 1.64019128])}
```

## 1.8 Shots VQE: Variance

[20]:
```
from qiskit_aer.primitives import Estimator as AerEstimator

aer_estimator = AerEstimator(run_options={"shots": 10000})

def evaluate_var(x0):
    estimator_job1 = aer_estimator.run(bethe.assign_parameters({kparts: x0}),␣
 ↪hamsquared)
    estimator_result1  = estimator_job1.result()
    estimator_job2 = aer_estimator.run(bethe.assign_parameters({kparts: x0}),␣
 ↪ham)
    estimator_result2  = estimator_job2.result()
    er1=estimator_result1.values[0]
    er2=estimator_result2.values[0]
    var =  er1  -  er2**2
    return var
```

[21]:
```
from qiskit_algorithms.optimizers import COBYLA

cobyla = COBYLA()

x0=np.random.uniform(0,np.pi,bethe.num_parameters)

print(x0)
opt_result = cobyla.minimize(evaluate_var, x0)
print(opt_result)
```

```
[1.10613195 0.50820055]
{   'fun': -0.005485500624999973,
```

```
'jac': None,
'nfev': 35,
'nit': None,
'njev': None,
'x': array([3.01552665, 0.9955594 ])}
```
