# Supplementary material for: Estimating Bethe roots with VQE
Source: arXiv:2404.18244 source file (2024-08-11)
Supplement: Supplementary file 2 [file BetheVQEClosed_arxiv1.pdf]

# BetheVQEClosed\_arxiv1

April 28, 2024

## 1 Estimating Bethe roots for the closed spin-1/2 XXZ chain using VQE

```
[14]: pip install qiskit-nature
```

```
Requirement already satisfied: qiskit-nature in /opt/conda/lib/python3.10/site-  
packages (0.7.2)  
Requirement already satisfied: qiskit>=0.44 in /opt/conda/lib/python3.10/site-  
packages (from qiskit-nature) (1.0.2)  
Requirement already satisfied: qiskit-algorithms>=0.2.1 in  
/opt/conda/lib/python3.10/site-packages (from qiskit-nature) (0.3.0)  
Requirement already satisfied: scipy>=1.4 in /opt/conda/lib/python3.10/site-  
packages (from qiskit-nature) (1.12.0)  
Requirement already satisfied: numpy>=1.17 in /opt/conda/lib/python3.10/site-  
packages (from qiskit-nature) (1.23.5)  
Requirement already satisfied: psutil>=5 in /opt/conda/lib/python3.10/site-  
packages (from qiskit-nature) (5.9.4)  
Requirement already satisfied: setuptools>=40.1.0 in  
/opt/conda/lib/python3.10/site-packages (from qiskit-nature) (65.5.1)  
Requirement already satisfied: typing-extensions in  
/opt/conda/lib/python3.10/site-packages (from qiskit-nature) (4.9.0)  
Requirement already satisfied: h5py in /opt/conda/lib/python3.10/site-packages  
(from qiskit-nature) (3.7.0)  
Requirement already satisfied: rustworkx>=0.12 in  
/opt/conda/lib/python3.10/site-packages (from qiskit-nature) (0.14.0)  
Requirement already satisfied: sympy>=1.3 in /opt/conda/lib/python3.10/site-  
packages (from qiskit>=0.44->qiskit-nature) (1.11.1)  
Requirement already satisfied: dill>=0.3 in /opt/conda/lib/python3.10/site-  
packages (from qiskit>=0.44->qiskit-nature) (0.3.6)  
Requirement already satisfied: python-dateutil>=2.8.0 in  
/opt/conda/lib/python3.10/site-packages (from qiskit>=0.44->qiskit-nature)  
(2.8.2)  
Requirement already satisfied: stevedore>=3.0.0 in  
/opt/conda/lib/python3.10/site-packages (from qiskit>=0.44->qiskit-nature)  
(5.1.0)  
Requirement already satisfied: symengine>=0.11 in  
/opt/conda/lib/python3.10/site-packages (from qiskit>=0.44->qiskit-nature)  
(0.11.0)
```

Requirement already satisfied: six>=1.5 in /opt/conda/lib/python3.10/site-packages (from python-dateutil>=2.8.0->qiskit>=0.44->qiskit-nature) (1.16.0)  
 Requirement already satisfied: pbr!=2.1.0,>=2.0.0 in /opt/conda/lib/python3.10/site-packages (from stevedore>=3.0.0->qiskit>=0.44->qiskit-nature) (6.0.0)  
 Requirement already satisfied: mpmath>=0.19 in /opt/conda/lib/python3.10/site-packages (from sympy>=1.3->qiskit>=0.44->qiskit-nature) (1.2.1)  
 Note: you may need to restart the kernel to use updated packages.

[15]: `pip install qiskit_algorithms`

Requirement already satisfied: qiskit\_algorithms in /opt/conda/lib/python3.10/site-packages (0.3.0)  
 Requirement already satisfied: qiskit>=0.44 in /opt/conda/lib/python3.10/site-packages (from qiskit\_algorithms) (1.0.2)  
 Requirement already satisfied: scipy>=1.4 in /opt/conda/lib/python3.10/site-packages (from qiskit\_algorithms) (1.12.0)  
 Requirement already satisfied: numpy>=1.17 in /opt/conda/lib/python3.10/site-packages (from qiskit\_algorithms) (1.23.5)  
 Requirement already satisfied: rustworkx>=0.14.0 in /opt/conda/lib/python3.10/site-packages (from qiskit>=0.44->qiskit\_algorithms) (0.14.0)  
 Requirement already satisfied: sympy>=1.3 in /opt/conda/lib/python3.10/site-packages (from qiskit>=0.44->qiskit\_algorithms) (1.11.1)  
 Requirement already satisfied: dill>=0.3 in /opt/conda/lib/python3.10/site-packages (from qiskit>=0.44->qiskit\_algorithms) (0.3.6)  
 Requirement already satisfied: python-dateutil>=2.8.0 in /opt/conda/lib/python3.10/site-packages (from qiskit>=0.44->qiskit\_algorithms) (2.8.2)  
 Requirement already satisfied: stevedore>=3.0.0 in /opt/conda/lib/python3.10/site-packages (from qiskit>=0.44->qiskit\_algorithms) (5.1.0)  
 Requirement already satisfied: typing-extensions in /opt/conda/lib/python3.10/site-packages (from qiskit>=0.44->qiskit\_algorithms) (4.9.0)  
 Requirement already satisfied: symengine>=0.11 in /opt/conda/lib/python3.10/site-packages (from qiskit>=0.44->qiskit\_algorithms) (0.11.0)  
 Requirement already satisfied: six>=1.5 in /opt/conda/lib/python3.10/site-packages (from python-dateutil>=2.8.0->qiskit>=0.44->qiskit\_algorithms) (1.16.0)  
 Requirement already satisfied: pbr!=2.1.0,>=2.0.0 in /opt/conda/lib/python3.10/site-packages (from stevedore>=3.0.0->qiskit>=0.44->qiskit\_algorithms) (6.0.0)  
 Requirement already satisfied: mpmath>=0.19 in /opt/conda/lib/python3.10/site-packages (from sympy>=1.3->qiskit>=0.44->qiskit\_algorithms) (1.2.1)  
 Note: you may need to restart the kernel to use updated packages.

```
[16]: import qiskit

qiskit.version.get_version_info()
```

```
[16]: '1.0.2'
```

### 1.1 Function $f(w, k)$

Make the function  $f(w, k)$  for a given set of Bethe roots  $\vec{k}$

$$f(w, \vec{k}) = \sum_{\sigma \in S_M} \varepsilon(\sigma) A(k_{\sigma(1)}, \dots, k_{\sigma(M)}) e^{i \sum_{j=1}^M k_{\sigma(j)} x_j}$$

$$A(k_1, \dots, k_M) = \prod_{1 \leq j < l \leq M} s(k_l, k_j)$$

$$s(k, k') = 1 - 2\Delta e^{ik'} + e^{i(k+k')}$$

```
[17]: import numpy as np
import math
import itertools
np.set_printoptions(suppress=True)
np.set_printoptions(threshold=np.inf)
```

```
[18]: #mylist is a collection of permutations t of the numbers 0 to M-1
def mylist(M):
    return list(itertools.permutations(range(M)))

# inversion number of t=(0,1,2,...,M-1)
def inv(t):
    x=0
    for j in range(M):
        for i in range(j):
            if t[i]>t[j]:
                x=x+1
    return x

# sign of permutation t
def e(t):
    return (-1)**inv(t)

def s(k,kp):
    return 1-2*Delta*np.exp(1.j*kp)+np.exp(1.j*(k+kp))

# k=[k0,...,kM-1]
def A(k):
    x=1
```

```

    for l in range(len(k)):
        for j in range(l):
            x=x*s(k[l],k[j])
    return x

# permutes the bethe roots k into an order determined by t: [k0,k1,k2] -> [k1,k2,k0]
    ↪
def kperm(k,t):
    y=[]
    for i in t:
        y.append(k[i])
    return y

# positions of the ones in w
def positions(w):
    x=[]
    for i in range(len(w)):
        if w[i]==1:
            x.append(i+1) # positions run from 1 to L, not 0 to L-1
    return x

def f(w,k):
    x=positions(w)
    z=0
    for t in mylist(len(k)):
        y=kperm(k,t)
        v=0
        for i in range(len(k)):
            v=v+y[i]*x[i]
        v=np.exp(1.j*v)
        z=z+e(t)*A(y)*v
    return z

```

## 1.2 Bethe code

```

[19]: from qiskit import *
from qiskit import QuantumRegister
from qiskit import QuantumCircuit
from qiskit.circuit.library import RYGate
from qiskit.circuit.library import UGate
np.set_printoptions(suppress=True)
np.set_printoptions(threshold=np.inf)

```

### 1.3 Variational ansatz

```
[56]: L=4
      M=1
      Delta=2
```

```
[57]: from qiskit.circuit import ParameterVector
```

Among the “kparts” cells below, ONLY ONE CELL SHOULD BE RUN!

If you are searching for all real roots, only the first cell is run, etc.

```
[58]: # M real roots
      kparts = ParameterVector("kparts", M)
      k=kparts
```

```
[11]: # one complex conjugate pair, M=2
      kparts = ParameterVector("kparts", 2)
      k=[kparts[0]+1j*kparts[1],kparts[0]-1j*kparts[1]]
```

```
[12]: # one complex pair, one real root, M=3
      kparts = ParameterVector("kparts", 3)
      k=[kparts[0]+1j*kparts[1],kparts[0]-1j*kparts[1],kparts[2]]
```

### 1.4 Bethe Circuit

Prepares the Bethe state

$$|B_M^L(\vec{k})\rangle = \sum_{w \in P(L,M)} f(w, \vec{k}) |w\rangle$$

```
[59]: q=QuantumRegister(L)
      bethe = QuantumCircuit(q)

      # Create set of permutations
      def P(L,M):
          if M==0:
              return [[0] * L]
          elif L-M==0:
              return [[1] * L]
          else:
              x=[]
              for p0 in P(L-1,M):
                  x.append(p0+[0])
              for p1 in P(L-1,M-1):
                  x.append(p1+[1])
              return x

      # store the coefficients f(w,k)
```

```

farray=[]
for w in P(L,M):
    farray=farray+[[w,f(w,k)]]

def F(b):
    sol=[] # solutions of w=ab
    for w in P(L,M):
        if w[L-len(b):L]==b:
            sol.append(w)
    if len(sol)==1:
        position=P(L,M).index(sol[0])
        return farray[position][1]
    else:
        x=0
        for p in sol:
            position=P(L,M).index(p)
            x=x+abs(farray[position][1])**2
        return x**0.5

def G(i,b):
    x=[i] + b
    return F(x)/F(b)

# a way of obtaining the angle arg(x) when x is a ParameterExpression
def myangle(x):
    eps=1e-16j
    y = -1j*np.log(x/np.abs(x)+eps)
    return (y+np.conjugate(y))/2

def theta(b):
    return 2*np.arccos(abs(G(1,b)))
def lam(b):
    return myangle(G(0,b)) -np.pi
def phi(b):
    return myangle(G(1,b))-lam(b)

def u(b):
    t=theta(b)
    la=lam(b)
    p=phi(b)
    return UGate(t,p,la)

def applyX(m,l):
    bethe.cx(L-m,L-m+1)

def applyI(m,l):
    sol=[] # these will be the strings b in P(L-m,M-l)

```

```

for b in P(L-m,M-1):
    if F(b)!=0: # Check that F(b)!=0
        sol.append(b)
if len(sol)==1:
    applyX(m,1)
    b=sol[0] # when b is unique, no extra controls are needed
    if l==1:
        cU = u(b).control(1)
        bethe.append(cU, [L-m+1,L-m])
    else:
        ccU = u(b).control(2)
        bethe.append(ccU, [L-m+1-1,L-m+1,L-m])
    applyX(m,1)
elif len(sol)>1:
    applyX(m,1)
    for b in sol:
        extra=[] # these are going to be the locations of the extra controls
        for i in range(len(b)):
            if b[i]==1:
                # if b=[0,1] then extra=[0], location of control
                extra.append(len(b)-i-1)
            if l==1:
                cU = u(b).control(1+len(extra))
                bethe.append(cU,extra + [L-m+1,L-m])
            else:
                ccU = u(b).control(2+len(extra))
                bethe.append(ccU,extra + [L-m+1-1,L-m+1,L-m])
        applyX(m,1)

# Create initial state
for i in range(M):
    bethe.x(i)
bethe.barrier()

# Apply I-gates
for m in reversed(range(2,L+1)):
    for l in range(max(M+m-L,1),min(M,m-1)+1):
        print(m,l)
        applyI(m,l)
        bethe.barrier()

#bethe.draw(output='mpl', initial_state=True)

```

```

4 1
3 1
2 1

```

## 1.5 Hamiltonian

$$\mathcal{H} = \frac{1}{4} \sum_{n=1}^L (\sigma_n^x \sigma_{n+1}^x + \sigma_n^y \sigma_{n+1}^y + \Delta \sigma_n^z \sigma_{n+1}^z) , \quad \vec{\sigma}_{L+1} = \vec{\sigma}_1$$

```
[60]: from qiskit_nature.second_q.hamiltonians.lattices import (
        BoundaryCondition,
        Lattice,
        LatticeDrawStyle,
        LineLattice,
    )
    from qiskit_nature.second_q.hamiltonians import HeisenbergModel

    from qiskit_nature.second_q.mappers import LogarithmicMapper

[61]: num_nodes=L
    hamop = HeisenbergModel(LineLattice(num_nodes,□
        ↪boundary_condition=BoundaryCondition.PERIODIC), (1.0, 1.0, Delta), (0.0, 0.
        ↪0, 0.0))
    hamop.second_q_op()
    logmapper = LogarithmicMapper()
    ham=logmapper.map(hamop.second_q_op())
    hamsquared = ham @ ham

[50]: #print(ham)
    #ham.to_matrix()
```

Prints the minimum eigenvalue of our Hamiltonian

```
[62]: from qiskit_algorithms import NumPyMinimumEigensolver

    numpy_solver = NumPyMinimumEigensolver()
    result = numpy_solver.compute_minimum_eigenvalue(operator=ham)
    ref_value = result.eigenvalue.real
    print(ref_value)

-2.7320508075688794
```

## 1.6 Statevector VQE: Ground state

```
[50]: from qiskit.primitives import Estimator
    from qiskit_algorithms.utils import algorithm_globals
    from qiskit_aer.primitives import Estimator as AerEstimator

    estimator = Estimator()

    # define optimizer
    from qiskit_algorithms.optimizers import SLSQP, COBYLA
```



```

iterations = 1000
optimizer = SLSQP(maxiter=iterations)
cobyla= COBYLA(maxiter=1000)

from qiskit_algorithms import VQE
# define callback
# note: Re-run this cell to restart lists before training
counts = []
values = []

def store_intermediate_result(eval_count, parameters, mean, std):
    counts.append(eval_count)
    values.append(mean)

```

```

[53]: x0=np.random.uniform(-np.pi,np.pi,bethe.num_parameters)

print(x0)

vqe = VQE(estimator, bethe, cobyla, callback=store_intermediate_result,
↪initial_point=x0)
result = vqe.compute_minimum_eigenvalue(operator=ham)

print(result)

[-2.29707071  2.16579033]
{  'aux_operators_evaluated': None,
   'cost_function_evals': 49,
   'eigenvalue': -2.7320507900528614,
   'optimal_circuit': <qiskit.circuit.quantumcircuit.QuantumCircuit object at
0x7fd16c874d90>,
   'optimal_parameters': {  ParameterVectorElement(kparts[0]):
-1.9454805743415615,
                           ParameterVectorElement(kparts[1]):
1.9454630239435262},
   'optimal_point': array([-1.94548057,  1.94546302]),
   'optimal_value': -2.7320507900528614,
   'optimizer_evals': None,
   'optimizer_result': <qiskit_algorithms.optimizers.optimizer.OptimizerResult
object at 0x7fd16bc24d60>,
   'optimizer_time': 1.3913002014160156}

```

## 1.7 Statevector VQE: Variance

```

[63]: # define Estimator for exact statevector simulation
from qiskit.primitives import StatevectorEstimator as Estimator

estimator = Estimator()

```

```

# define optimizer
from qiskit_algorithms.optimizers import SLSQP, COBYLA
iterations = 1000
optimizer = SLSQP(maxiter=iterations)
cobyla= COBYLA(maxiter=1000)

from qiskit_algorithms import VQE

```

```

[65]: def evaluate_var(params):
    estimator_job1 = estimator.run([(bethe, hamsquared, params)])
    estimator_job2 = estimator.run([(bethe, ham, params)])
    estimator_result1 = estimator_job1.result()
    estimator_result2 = estimator_job2.result()
    er1=estimator_result1[0].data.evs
    er2=estimator_result2[0].data.evs
    var = er1 - er2**2
    return var

x0=np.random.uniform(-np.pi,np.pi,bethe.num_parameters)
print(x0)
opt_result = cobyla.minimize(evaluate_var, x0)
print(opt_result)

```

```

[0.05504591]
{  'fun': 9.836683245723066e-09,
   'jac': None,
   'nfev': 21,
   'nit': None,
   'njev': None,
   'x': array([0.00007013])}

```

## 1.8 Shots VQE: Ground state

```

[54]: from qiskit_aer.primitives import Estimator as AerEstimator

aer_estimator = AerEstimator(run_options={"shots": 10000})

def evaluate_energy(x0):
    estimator_job1 = aer_estimator.run(bethe.assign_parameters({k: x0}), ham)
    estimator_result1 = estimator_job1.result()
    return estimator_result1.values

```

```

[55]: from qiskit_algorithms.optimizers import COBYLA

cobyla = COBYLA()

```

```

x0=np.random.uniform(-np.pi,np.pi,bethe.num_parameters)
print(x0)
opt_result = cobyala.minimize(evaluate_energy, x0)
print(opt_result)

```

```

[ 3.10871429 -2.5422158 ]
{  'fun': -2.7029,
   'jac': None,
   'nfev': 31,
   'nit': None,
   'njev': None,
   'x': array([ 2.01950078, -2.00694743])}

```

## 1.9 Shots VQE: Variance

```

[66]: from qiskit_aer.primitives import Estimator as AerEstimator

aer_estimator = AerEstimator(run_options={"shots": 10000})

def evaluate_var(x0):
    estimator_job1 = aer_estimator.run(bethe.assign_parameters({kparts: x0}),
    ↪hamsquared)
    estimator_result1 = estimator_job1.result()
    estimator_job2 = aer_estimator.run(bethe.assign_parameters({kparts: x0}),
    ↪ham)
    estimator_result2 = estimator_job2.result()
    er1=estimator_result1.values[0]
    er2=estimator_result2.values[0]
    var = er1 - er2**2
    return var

```

```

[72]: from qiskit_algorithms.optimizers import COBYLA

cobyala = COBYLA()

x0=np.random.uniform(-np.pi,np.pi,bethe.num_parameters)
print(x0)
opt_result = cobyla.minimize(evaluate_var, x0)
print(opt_result)

```

```

[-0.03605381]
{  'fun': -0.00121855999999999797,
   'jac': None,
   'nfev': 18,
   'nit': None,
   'njev': None,
   'x': array([-0.06740381])}

```
